# Supplementary material for: Geometric Insights into Focal Loss: Reducing Curvature for Enhanced Model Calibration
Source: arXiv:2405.00442 source file (2024-05-01)
Supplement: Supplementary file 1 [file A_nn_geometry.tex]

\section{Geometry of neural networks}
\label{apd:geometry}
Throughout the manuscript, the Einstein summation convention is assumed, so that summation will be automatically taken over indices repeated twice in the term, e.g., $\bm{a}^i\bm{b}_i = \sum_{i} a^ib_i$.

\begin{example}[Manifold of one-layer neural networks]
    \label{example:one_layer_nn}
    As an example, we now consider a one-layer neural network with sigmoid function $\sigma(z)=1/(1+e^{-z})$.
    Let $\bm{x}\in\mathbb{R}^d$ be an $n$-dimensional input and $y=\sigma(\bm{\theta}^T\bm{x} + \theta_0)$ be the one-dimensional output, where $\bm{\theta}\in\mathbb{R}^d$ and $\theta_0\in\mathbb{R}$ are the weights and the bias.
    Then the set of outputs
    \begin{align*}
        \mathcal{H}_\sigma &= \{h(\bm{x}; \bm{\theta}, \theta_0)\ |\ \bm{\theta}\in\mathbb{R}^d, \theta_0 \in\mathbb{R}\} \\
        &= \{\sigma(\bm{\theta}^T\bm{x} + \theta_0)\ | \bm{\theta}\in\mathbb{R}^d, \theta_0\in\mathbb{R}\}
    \end{align*}
    can be regarded as an $(d+1)$-dimensional manifold, parameterized by $\bm{\theta}$ and $\theta_0$.
    
    In practice, we can verify that the Jacobian matrix of $y=y(\bm{\theta}, \theta_0)$ are full-rank:
    From the properties of the sigmoid function, we have
    \begin{align*}
        \frac{\partial y}{\partial \theta_0} &= \sigma'(\bm{\theta}^T\bm{x} + \theta_0) = y(1-y), \\
        \frac{\partial y}{\partial \theta_j} &= \sigma'(\bm{\theta}^T\bm{x} + \theta_0)x_j = y(1-y)x_j.
    \end{align*}
    Then, for $a_0, a_1,\dots,a_n\in\mathbb{R}$, let $a_0\frac{\partial y}{\partial \theta_0} + \sum^d_{j=1}a_j\frac{\partial y}{\partial \theta_j} = 0$.
    Since $y(1-y)\neq 0$ for finite $\bm{\theta}^\top\bm{x} + \theta_0$, the previous relation becomes $a_0 + \sum^d_{j=1}a_jx_j = 0$.
    Since this relation holds for any $x_j\in\mathbb{R}$, it follows that $a_0=a_1=\cdots=a_n=0$.
    Therefore, $\{\frac{\partial y}{\partial \theta_0}, \frac{\partial y}{\partial \theta_1},\dots,\frac{\partial y}{\partial \theta_d}\}$ are linearly independent, hence the rank of Jacobian of $y$ is $d+1$.
    This means that the set of neural networks forms a manifold with parameters as its coordinate system.
\end{example}
In general, neural networks or families of probability distributions construct Riemannian (non-Euclidean) manifolds. In this section, we organize the geometric concepts used in this paper.
For more details, see textbooks on Riemannian manifolds and differential geometry~\cite{lee2018introduction,kuhnel2015differential,guggenheimer2012differential,lee2006riemannian}.

\begin{definition}
    \label{def:chart}
    Let $U \subset \mathcal{M}$ be an open set.
    Then the pair $(U, \phi)$ is called a chart (coordinate system) on $\mathcal{M}$, if $\phi: U \to \phi(U) \subset \mathbb{R}^d$ is a homeomorphism of the open set $U$ in $\mathcal{M}$ onto an open set $\phi(U)$ of $\mathbb{R}^d$.
    The coordinate functions on $U$ are defined as $\theta^j: U \to \mathbb{R}$, and $\phi(p) = (\theta^1(p), \theta^2(p),\dots, \theta^d(p))$, namely $\theta^i = u^i \circ \phi$, where $u^i: \mathbb{R}^d \to \mathbb{R}$, $u^i(a_1,\dots,a_d) = a_i$ is the $i$-th projection.
\end{definition}
\begin{definition}
    \label{def:atlas}
    An atlas $\mathcal{A}$ of dimension $d$ associated with the metric space $\mathcal{M}$ is a collection of charts $\{U_\alpha, \phi_\alpha\}$ such that
    \begin{itemize}
        \item[i)] $U_\alpha \subset \mathcal{M}, \bigcup_\alpha U_\alpha = \mathcal{M}$;
        \item[ii)] if $U_\alpha \cap U_\beta \neq \emptyset$, the restriction to $\phi_\alpha(U_\alpha \cap U_\beta)$ of the map
        \begin{align*}
            F_{\alpha\beta} \coloneqq \phi_\beta \circ \phi_\alpha^{-1} : \phi_\alpha(U_\alpha \cap U_\beta) \to \phi_\beta(U_\alpha \cap U_\beta)
        \end{align*}
        is differentiable from $\mathbb{R}^d$ to $\mathbb{R}^d$.
    \end{itemize}
\end{definition}
\begin{definition}
    \label{def:manifold}
    A differentiable manifold $\mathcal{M}$ is a metric space endowed with a complete atlas.
    The dimension $d$ of the atlas is called the dimension of the manifold.
\end{definition}
\begin{definition}
    \label{def:differentiable_function}
    A function $f: \mathcal{M} \to \mathbb{R}$ is said to be differentiable if for any chart $(U, \phi)$ on $\mathcal{M}$ the function $f \circ \phi^{-1}: \phi(U) \to \mathbb{R}$ is differentiable.
    The set of all differentiable functions on the manifold $\mathcal{M}$ is denoted by $\mathcal{F}(\mathcal{M})$.
\end{definition}
\begin{definition}
    \label{def:tangent_space}
    The set of all tangent vectors at $p \in \mathcal{M}$ to $\mathcal{M}$ is called the tangent space of $\mathcal{M}$ at $p$, and is denoted by $T_p\mathcal{M}$.
\end{definition}
\begin{definition}
    \label{def:lie_bracket}
    The Lie bracket, which is given by $[ \ ,\ ] : \mathcal{X}(\mathcal{M})\times\mathcal{X}(\mathcal{M}) \to \mathcal{X}(\mathcal{M})$, is defined as
    \begin{align*}
        [X, Y]_pf \coloneqq X_p(Yf) - Y_p(Xf), \quad \forall f \in \mathcal{F}(\mathcal{M}), p \in \mathcal{M}.
    \end{align*}
\end{definition}
\begin{definition}
    \label{def:riemannian_manifold}
    A Riemannian metric $\mathfrak{g}$ on a differentiable manifold $\mathcal{M}$ is a symmetric, positive definite $2$-covariant tensor field.
    A Riemannian manifold is a differentiable manifold $\mathcal{M}$ endowed with a Riemannian metric $\mathfrak{g}$.
\end{definition}
A Riemannian manifold is denoted by the pair $(\mathcal{M}, \mathfrak{g})$, and $\mathfrak{g}$ can be considered as a positive definite scalar product $\mathfrak{g}_p: T_p\mathcal{M} \times T_p\mathcal{M} \to \mathbb{R}$ that depends differentially on the point $p \in \mathcal{M}$.
In local coordinates, $\mathfrak{g}$ can be written as
\begin{align*}
    \mathfrak{g} = \mathfrak{g}_{ij}d\theta_id\theta_j
\end{align*}
with $\mathfrak{g}_{ij} = \mathfrak{g}_{ji} = \mathfrak{g}(\frac{\partial}{\partial\theta_i}, \frac{\partial}{\partial\theta_j})$, and $\mathfrak{g}(X, Y) = \mathfrak{g}_{ij}X^iY^j$ for a pair of vector fields $(X, Y)$.

\begin{definition}
    \label{def:linear_connection}
    A linear connection $\nabla$ on a differentiable manifold $\mathcal{M}$ is a map $\nabla: \mathcal{X}(\mathcal{M}) \times \mathcal{X}(\mathcal{M}) \to \mathcal{X}(\mathcal{M})$ with the following properties:
    \begin{itemize}
        \item[i)] $\nabla_XY$ is $\mathcal{F}(\mathcal{M})$-linear in $X$;
        \item[ii)] $\nabla_XY$ is $\mathbb{R}$-linear in $Y$;
        \item[iii)] it satisfies the Leibniz rule
        \begin{align*}
            \nabla_X(fY) = (Xf)Y + f\nabla_XY,\quad \forall f \in \mathcal{F}(\mathcal{M}).
        \end{align*}
    \end{itemize}
\end{definition}
\begin{definition}
    \label{def:metric_connection}
    Let $\mathfrak{g}$ be the Riemannian metric tensor.
    A linear connection $\nabla$ is called metric connection if $\mathfrak{g}$ is parallel with respect to $\nabla$, that is,
    \begin{align}
        \nabla_Z\mathfrak{g} = 0, \quad \forall Z \in \mathcal{X}(\mathcal{M}).
    \end{align}
\end{definition}

The next theorem provides the Levi-Civita connection as an explicit expression in terms of the Riemannian metric $\mathfrak{g}$.
\begin{theorem}
    \label{thm:levi_civita_connection}
    On a Riemannian manifold, there exists a unique torsion-free, metric connection $\nabla$.
    Furtheremore, $\nabla$ is given by the following Koszul formula
    \begin{align}
        2\mathfrak{g}(\nabla_XY, Z) &= X\mathfrak{g}(Y, Z) + Y\mathfrak{g}(X, Z) - Z\mathfrak{g}(X, Y) \nonumber \\
        &+ \mathfrak{g}([X, Y], Z) - \mathfrak{g}([X, Z], Y) - \mathfrak{g}([Y, Z], X). \label{eq:levi_civita_connection}
    \end{align}
\end{theorem}
\begin{proof}
    The proof includes the existence and uniqueness.

    (Existence) It suffices to show that $\nabla$ defined by \eqref{eq:levi_civita_connection} is a metric and torsion-free connection.
    First, using the properties of vector fields and Lie brackets,
    \begin{align*}
        2\mathfrak{g}(\nabla_{fX}Y, Z) = 2f\mathfrak{g}(\nabla_XY, Z), \quad \forall Z \in \mathcal{X}(\mathcal{M}),
    \end{align*}
    and $\nabla_{fX}Y = f\nabla_XY, \forall X, Y \in \mathcal{X}(\mathcal{M})$, that is, $\nabla$ is $\mathcal{F}(\mathcal{M})$-linear in the first argument.
    Next,
    \begin{align*}
        2\mathfrak{g}(\nabla_X(fY), Z) &= X\mathfrak{g}(fY, Z) + fY\mathfrak{g}(X, Z) - Z\mathfrak{g}(X, fY) \\
        &+ \mathfrak{g}([X, fY], Z) - \mathfrak{g}([X, Z], fY) \\
        &- \mathfrak{g}([fY, Z], X) \\
        &= X(f)\mathfrak{g}(Y, Z) + fX\mathfrak{g}(Y, Z) + fY\mathfrak{g}(X, Z) \\
        &- Z(f)\mathfrak{g}(X, Y) - fZ\mathfrak{g}(X, Y) \\
        &+ f\mathfrak{g}([X, Y], Z) + X(f)\mathfrak{g}(Y, Z) \\
        &- f\mathfrak{g}([X, Z], Y) \\
        &- f\mathfrak{g}([Y, Z], X) + Z(f)\mathfrak{g}(Y, X) \\
        &= 2f\mathfrak{g}(\nabla_XY, Z) + 2X(f)\mathfrak{g}(Y, Z) \\
        &= 2\mathfrak{g}(f\nabla_XY + X(f)Y, Z).
    \end{align*}
    This yields Leibniz formula, and $\nabla$ is a linear connection.
    We also have
    \begin{align*}
        2\mathfrak{g}(T(X, Y), Z) &= 2\mathfrak{g}(\nabla_XY, Z) - 2\mathfrak{g}(\nabla_YX, Z) \\
        &- 2\mathfrak{g}([X, Y], Z) \\
        &= X\mathfrak{g}(Y, Z) + Y\mathfrak{g}(X, Z) - Z\mathfrak{g}(X, Y) \\
        &+ \mathfrak{g}([X, Y], Z) - \mathfrak{g}([X, Z], Y) - \mathfrak{g}([Y, Z], X) \\
        &- Y\mathfrak{g}(X, Z) - X\mathfrak{g}(Y, Z) + Z\mathfrak{g}(Y, X) \\
        &- \mathfrak{g}([Y, X], Z) + \mathfrak{g}([Y, Z], X) + \mathfrak{g}([X, Z], Y) \\
        &- 2\mathfrak{g}([X, Y], Z) \\
        &= \mathfrak{g}(2[X, Y] - 2[X, Y], Z) = 0.
    \end{align*}
    This implies that torsion tensor $T(X, Y) = 0$, for all $X, Y \in \mathcal{X}(\mathcal{M})$.
    Then, 
    \begin{align*}
        & 2\mathfrak{g}(\nabla_ZX, Y) + 2\mathfrak{g}(X, \nabla_ZY) \\
        &= Z\mathfrak{g}(X, Y) + X\mathfrak{g}(Z, Y) - Y\mathfrak{g}(Z, Y) - Y\mathfrak{g}(Z, X) \\
        &+ \mathfrak{g}([Z, X], Y) - \mathfrak{g}([Z, Y], X) - \mathfrak{g}([X, Y], Z) \\
        &+ Z\mathfrak{g}(Y, X) + Y\mathfrak{g}(Z, X) - X\mathfrak{g}(Z, Y) + \mathfrak{g}([Z, Y], X) \\
        &- \mathfrak{g}([Z, X], Y) - \mathfrak{g}([Y, X], Z) \\
        &= 2Z\mathfrak{g}(X, Y).
    \end{align*}
    Therefore, $\mathfrak{g}(\nabla_ZX, Y) + \mathfrak{g}(X, \nabla_ZY) = Z\mathfrak{g}(X, Y)$ and $\nabla$ is a metric connection.

    (Uniqueness) It suffices to show that any metric and symmetric connection $\nabla$ is given by \eqref{eq:levi_civita_connection}.
    We consider the local coordinate sysmte $(\theta^1,\dots,\theta^d).$
    Let $X = \frac{\partial}{\partial\theta_i}$, $Y = \frac{\partial}{\partial\theta_j}$, $Z = \frac{\partial}{\partial\theta_k}$.
    By $\Gamma^k_{ij} = \mathfrak{g}(\nabla_{\frac{\partial}{\partial\theta_i}}\frac{\partial}{\partial\theta_j}, \frac{\partial}{\partial\theta_k})$ and $\mathfrak{g}_{ij} = \mathfrak{g}(\frac{\partial}{\partial\theta_i}, \frac{\partial}{\partial\theta_j})$,
    \begin{align*}
        2\Gamma^l_{ij}\mathfrak{g}_{lk} = \frac{\partial}{\partial\theta_i}\mathfrak{g}_{jk} + \frac{\partial}{\partial\theta_j}\mathfrak{g}_{ik} - \frac{\partial}{\partial\theta_k}\mathfrak{g}_{ij}.
    \end{align*}
    Since $\nabla$ is a metric connection, we have
    \begin{align*}
        \frac{\partial}{\partial\theta_i}\mathfrak{g}_{jk} &= \Gamma^l_{ij}\mathfrak{g}_{lk} + \Gamma^m_{ik}\mathfrak{g}_{jm}, \\
        \frac{\partial}{\partial\theta_j}\mathfrak{g}_{ki} &= \Gamma^l_{jk}\mathfrak{g}_{li} + \Gamma^m_{ji}\mathfrak{g}_{km}, \\
        \frac{\partial}{\partial\theta_k}\mathfrak{g}_{ij} &= \Gamma^l_{ki}\mathfrak{g}_{lj} + \Gamma^m_{kj}\mathfrak{g}_{im},
    \end{align*}
    and by using the symmetry $\Gamma^k_{ij} = \Gamma^k_{ji}$, we can confirm the uniqueness.
\end{proof}

We can also define the following dualistic structure.
\begin{definition}
    \label{def:dual_connections}
    Let $(\mathcal{M}, \mathfrak{g})$ be a Riemannian manifold.
    Two connections $\nabla$ and $\nabla^*$ on $\mathcal{M}$ are called dual, with respect to the metric $\mathfrak{g}$, if
    \begin{align}
        Z\mathfrak{g}(X, Y) = \mathfrak{g}(\nabla_ZX, Y) + \mathfrak{g}(X, \nabla^*_ZY),
    \end{align}
    for all $X, Y, Z \in \mathcal{X}(\mathcal{M})$.
\end{definition}
This notion yields the dual Hessian, which is used in Theorem~\ref{thm:curvature_contractions}.

% example of NN manifold
% indicates non-Euclidean

% Def. Riemmanian manifold
% Def. Curvature
