# Supplementary material for: Geometric Insights into Focal Loss: Reducing Curvature for Enhanced Model Calibration
Source: arXiv:2405.00442 source file (2024-05-01)
Supplement: Supplementary file 2 [file C_additional_discussion.tex]

\section{Additional discussions}
\label{apd:additional_discussions}
Here, we dive into further additional discussions based on a geometric perspective.

\subsection{OOD generalization and curvature}
\label{apd:additional_discussion_ood_curvature}
In this work, we focus our discussion on SAM and focal loss. However, relevant discussions are expected to be extended to other algorithms as well.
For example, Fishr~\cite{rame2022fishr}, which has achieved state-of-the-art or comparable performance in out-of-distribution generalization, reports important discussions regarding the direction of the maximum eigenvalue of the Hessian.
It is known that other OOD algorithms~\cite{kim2021locally,parker2020ridge} also depend on the eigenvectors of Hessian.

\subsection{Other contractions of curvature}
\label{apd:additional_discussion_other_curvature}
In this work, we consider the spectral radius and Laplacian as measures of curvature contraction.
However, besides these, several alternative contractions of curvature can be considered, which can also provide further insights.
One alternative is the operator norm of Hessian $\|H^f\|_p = \max_{\bm{x} \neq 0}\|H^f\bm{x}\|_p / \|\bm{x}\|_p$.
It satisfies that
\begin{align}
    \|H^f\|_p \geq A(H^f)
\end{align}
for arbitrary $p$ and
\begin{align}
    \lim_{p\to\infty} \|H^{fp}\|^{1/p} = A(H^f).
\end{align}
Existing work~\cite{kimura2022information} discusses the relation between the behavior of dropout~\cite{JMLR:v15:srivastava14a} and the norm of Fisher information matrix.

Another alternative is the following Gaussian curvature.
\begin{definition}[Gaussian curvature]
   \label{def:gaussian_curvature} 
   The Gaussian curvature $K(H^f)$ of $f\in\mathcal{F}(\mathcal{M})$ is defined as the product of principal curvatures and can be given as
   \begin{align}
       K(H^f) \coloneqq \det(H^f).
   \end{align}
\end{definition}
From fact that
\begin{align*}
    \det(H^f) = \prod_{i=1}\lambda_i,
\end{align*}
for eigenvalues $\lambda_i$ of $H^f$, we can relate Gaussian curvature with spectral radius and Laplacian.
We can also use this alternative to understand the behavior of machine learning algorithms.
For example, it is known that SGD with isotropic noise avoids sharp minima by increasing the determinant of the Hessian~\cite{jastrzkebski2017three}.
This implies that the corresponding optimization strategy depends on the Gaussian curvature $K(H^f)$.
Moreover, the metric tensor $\mathfrak{g}$ in the statistical manifold is Fisher information matrix and is Hessian of the negative log-likelihood function
\begin{align}
    \mathfrak{g}_{ij} = -\frac{\partial^2}{\partial\theta_i\partial\theta_j}\ell(\bm{\theta}),
\end{align}
where $\ell(\bm{\theta}) = \ln p(\bm{x};\bm{\theta})$.
The determinant of metric $\mathfrak{g}$ is also known as the Riemannian volume element $dv$ as
\begin{align}
    dv = \sqrt{\det{\mathfrak{g}}}\ d\theta^1\land\cdots\land d\theta^d. \label{eq:riemannian_volume_element}
\end{align}
More precisely, for any point $p \in \mathcal{M}$, let $\{e_i; i=1,\dots,n\}_p$ be an orthonormal basis in $T_p\mathcal{M}$, with respect to the metric $\mathfrak{g}$, and $\{e^*_i\}$ be the associated dual basis as $e^*_i(e_j) = \delta^i_j$.
The Riemannian volume form $dv$ is defined by
\begin{align*}
    dv_{|p} \coloneqq e^*_1(p) \land \cdots \land e^*_n(p).
\end{align*}
For local basis $\{\partial / \partial\theta_i\}^d_{i=1}$, the Riemannian metric is given by
\begin{align*}
    \mathfrak{g}_{ij}(p) = \mathfrak{g}\left(\frac{\partial}{\partial\theta_i}(p), \frac{\partial}{\partial\theta_j}(p)\right).
\end{align*}
Let $\frac{\partial}{\partial\theta_i}(p) = b^k_i e^*_k$ with the matrix $B = (b^k_i)$, and we have
\begin{align*}
    & dv_p\left(\frac{\partial}{\partial\theta_1}(p),\dots,\frac{\partial}{\partial\theta_d}(p)\right) \\
    &= e^*_1(p)\land\cdots\land e^*_d(p)\left(\frac{\partial}{\partial\theta_1}(p),\dots,\frac{\partial}{\partial\theta_d}(p)\right) \\
    &= \det\left(e^*_i\left(\frac{\partial}{\partial\theta_i}(p)\right)\right) \\
    &= \det \mathfrak{g}_p\left(e^*_i, \frac{\partial}{\partial\theta_j}(p)\right) \\
    &= \det \mathfrak{g}_p\left(e^*_i, b^k_je^*_k\right) \\
    &= \det\left(b^k_j\mathfrak{g}_p(e^*_i, e^*_k)\right) \\
    &= \det(b^k_j\delta^i_k) = \det(b^i_j) = \det B.
\end{align*}
We also have
\begin{align*}
    \det(\mathfrak{g}_{ij}) &= \det \mathfrak{g}\left(\frac{\partial}{\partial\theta_i}(p), \frac{\partial}{\partial\theta_j}(p)\right) \\
    &= \det\left(b^k_ib^l_j\mathfrak{g}(e^*_k, e^*_l)\right) \\
    &= \det(b^k_ib^l_j\delta_{kl}) \\
    &= \det(BB^\top) = (\det B)^2.
\end{align*}
Then, these yield \eqref{eq:riemannian_volume_element}.
It is worth nothing that Jeffrey's prior~\cite{jeffreys1998theory,jeffreys1946invariant} in Bayesian statistics is the parallel volume form with respect to the Levi-Civita connection of the Fisher metric.
For general $\alpha \in \mathbb{R}$, the later works~\cite{takeuchi2005spl,matsuzoe2006equiaffine} consider the $\alpha$-parallel prior, which is a volume form that is parallel with respect to the $\nabla^{(\alpha)}$ connection, and $\alpha = 0$ recovers Jeffrey's prior from Bayesian inference.
Other work~\cite{kimura2022igiwerm,kimura2021alpha,kimura2021generalized} provide the relationship between the choice of learning algorithm and the Riemannian skewness tensor.
