# Supplementary material for: Geometric Insights into Focal Loss: Reducing Curvature for Enhanced Model Calibration
Source: arXiv:2405.00442 source file (2024-05-01)
Supplement: Supplementary file 3 [file D_exp_setting.tex]

\begin{table*}[tbh]
\centering
\newcolumntype{P}[1]{>{\centering\arraybackslash}p{#1}}
\begin{tabular}{llllllP{8em}l}
\toprule
Model & $\mathcal{L}$ & Dataset & Optimizer & $\eta$ & $B$  & $\rho$ or $\gamma$ & Epochs Budget\\
\midrule
ResNet-18  & Focal Loss & CIFAR10 & MomentumSGD  & [0.01] & 256 & [10.0, 5.0, 2.0, 1.5, 1.0, 0.75, 0.5, 0.25, 0.1] &200\\ 
ResNet-18  & Cross Entropy & CIFAR10 & SAM  & [0.01] & 256 & [0.5, 0.1, 0.05, 0.01, 0.001, 0.0001, 0.00001, 0] &200\\ 
ResNet-50  & Focal Loss & CIFAR10 & MomentumSGD  & [0.1] & 256 & [10.0, 5.0, 2.0, 1.5, 1.0, 0.75, 0.5, 0.25, 0.1, 0] &90\\ 
ResNet-50  & Cross Entropy & CIFAR10 & SAM  & [0.1] & 256 & [5, 1, 0.5, 0.1, 0.05, 0.01, 0.005] &90\\ 
\hline
\end{tabular}\\ 
\caption{CIFAR10 $\to$ CIFAR10.1 and ImageNet-1K $\to$ ImageNet-V2 Tasks: Hyperparameter}
\label{tab:exp_cifar_in}
% }
\end{table*}

\begin{table*}[tbh]
\centering
\newcolumntype{P}[1]{>{\centering\arraybackslash}p{#1}}
\begin{tabular}{llllP{3em}lP{8em}l}
\toprule
Model & $\mathcal{L}$ & Dataset & Optimizer & $\eta$ & $B$  & $\rho$ & Epochs Budget\\
\midrule
ResNet-18  & Cross Entropy & CIFAR10 & SAM  & [0.00025, 0.00001] & 1 & [0.5, 0.1, 0.05, 0.01, 0.001, 0.0001, 0.00001, 0] &200\\ 
ResNet-18  & Cross Entropy & CIFAR10 & SAM  & [0.01] & 256 & [0.5, 0.1, 0.05, 0.01, 0.001, 0.0001, 0.00001, 0] &200\\ 
ResNet-18  & Cross Entropy & CIFAR10 & SAM  & [0.01] & 40000 & [0.5, 0.1, 0.05, 0.01, 0.001, 0.0001, 0.00001, 0] &1000\\ 
\hline
\end{tabular}\\ 
\caption{CIFAR10 $\to$ CIFAR10.1 Task / Batch Size Comparison: Hyperparameter}
\label{tab:exp_cifar_bs}
% }
\end{table*}

\begin{table*}[tbh]
\centering
\newcolumntype{P}[1]{>{\centering\arraybackslash}p{#1}}
\begin{tabular}{llllP{10em}lP{5em}l}
\toprule
Model & $\mathcal{L}$ & Dataset & Optimizer & $\eta$ & $B$  & $\rho$ & Steps Budget\\
\midrule
ResNet-50  & Cross Entropy & PACS & SAM & [0.5, 0.1, 0.05, 0.01, 0.005, 0.001, 0.0005, 0.0001] & 32 & [0.5, 0.1, 0.05, 0.01, 0.001, 0] & 5000\\ 
ResNet-50  & Cross Entropy & VLCS & SAM & [0.5, 0.1, 0.05, 0.01, 0.005, 0.001, 0.0005, 0.0001] & 32 & [0.5, 0.1, 0.05, 0.01, 0.001, 0] & 5000\\ 
ResNet-50  & Cross Entropy & OfficeHome & SAM & [0.5, 0.1, 0.05, 0.01, 0.005, 0.001, 0.0005, 0.0001] & 32 & [0.5, 0.1, 0.05, 0.01, 0.001, 0] & 5000\\ 
ResNet-50  & Cross Entropy & DomainNet & SAM & [0.5, 0.1, 0.05, 0.01, 0.005, 0.001, 0.0005, 0.0001] & 32 & [0.5, 0.1, 0.05, 0.01, 0.001, 0] & 5000\\

\hline
\end{tabular}\\ 
\caption{DomainBed Tasks: Hyperparameter}
\label{tab:exp_db}
% }
\end{table*}

\section{Experimental Setting}
\label{appendix:exp_setting}

\subsection{Overview}
In our experimental procedure, we adopted a rigorous grid search methodology to fine-tune the hyperparameters. This included adjusting the $\rho$ parameter for the SAM and $\eta$ for the Stochastic Gradient Descent optimizer, thus allowing us to uncover hyperparameter combinations that yield the most effective performance.

A detailed account of the batch size, total number of epochs allocated for each dataset, corresponding model, and the selection of $\rho$ for SAM and $\gamma$ for Focal Loss is meticulously presented in \cref{tab:exp_cifar_in},\ref{tab:exp_cifar_bs} and, \ref{tab:exp_db}. We carefully selected these parameters to promote optimal learning while minimizing the risk of overfitting. The ranges specified for these parameters were based on prior studies that sought to identify hyperparameters maximizing validation performance.

We use Momentum SGD as the default optimizer with a momentum factor set to $\beta=0.9$ in our experiments.

For the experiments employing a full batch, we acknowledged the possibility of insufficient update times, as the number of steps equates to the number of epochs. To address this, we set the epochs budget to 1000. Meanwhile, in the experiments where the batch size was set to 1, we hypothesized the potential of the loss function not being approximated adequately. To mitigate this issue, we carefully set a small learning rate, such as $[0.00025, 0.00001]$, and proceeded with our experiments.

\subsection{Models}

In our experiments, we employ two models from the ResNet architecture \cite{he2016deep}: ResNet-50 and ResNet-18.
Both models are well-established, broadly adopted, and demonstrate competitive performance across numerous tasks, making them excellent choices for our investigation.\\

\noindent
{\bf{ResNet-50}} \cite{he2016deep}\\
ResNet-50 is a 50-layer deep convolutional neural network that leverages skip-conection to train such deep models. ResNet-50 consists of a stack of 16 residual blocks, where each block contains three layers - one 1x1 convolution for dimensionality reduction, one 3x3 convolution, and another 1x1 convolution for restoring dimensionality. 
This arrangement forms a bottleneck structure which not only reduces the number of parameters but also mitigates overfitting. 
These blocks are followed by a global average pooling and a fully connected layer for classification.
For the task of domain generalization by using the DomainBed \cite{Gulrajani21} dataset, we use a pre-trained model of ResNet50 on the ImageNet-1K dataset \footnote{\url{https://download.pytorch.org/models/resnet50-0676ba61.pth}}.\\

\noindent
{\bf{ResNet-18}}\\
On the other hand, ResNet-18 is a lighter variant of the ResNet architecture and consists of a stack of 8 residual blocks. We use ResNet18 for the training task of CIFAR10.

\subsection{Datasets}

\noindent
{\bf{CIFAR10.1}} \cite{recht2018cifar10.1}\\
Approximately 2,000 fresh test images constitute this dataset, a product of research on the primary CIFAR-10 dataset. The compilation was judiciously planned to curtail distributional shifts. CIFAR-10.1's images form a subsection of the TinyImages dataset.\\

\noindent
{\bf{ImageNet-V2}} \cite{recht2019imagenet}\\
The ImageNet-V2 dataset is a modern benchmark for image recognition models, providing three test sets with 10,000 fresh images each. This dataset, which evolved over a decade from its original ImageNet dataset, avoids adaptive overfitting biases in accuracy assessments. Its data collection process mirrors the original ImageNet principles. Researchers are provided with ImageNet-V2 compatible code, a pool of candidate images, and detailed metadata. ImageNet-V2 divides into three categories: TopImages, Threshold0.7, and MatchedFrequency. Evaluations across all categories are averaged to report Test OOD accuracy and Test OOD ECE.\\

\noindent
{\bf{DomainBed}} \cite{Gulrajani21}\\
DomainBed serves as an all-encompassing benchmark for domain adaptation/generalization algorithms. It is envisioned as a standardized and diverse testbed that enables impartial comparisons of different methodologies. The specifics of the included datasets in DomainBed vary, each offering a distinct test for a domain adaptation algorithm's ability to generalize across different distributions. Despite DomainBed incorporating seven sub-datasets, we directed our experiments to primarily analyze SAM behavior for PACS \cite{li2017deeper}, VLCS \cite{fang2013unbiased}, OfficeHome \cite{venkateswara2017deep}, and DomainNet \cite{peng2019moment}.

\subsection{Hessian Calculation}

In our experimental setup, explicitly calculating the Hessian presents a challenge due to memory size limitations, particularly in practical problem settings. Consequently, we opted to use approximation calculations. More specifically, we utilized the calculation methods for Laplacian ($\mathrm{tr}(H^{f})$) and spectral radius (SR(H): $A(H^f)$) provided in PyHessian\footnote{\url{https://github.com/amirgholami/PyHessian}} \cite{Yao20}.

The Hutchinson method, a widely-used algorithm known for approximating the trace of the Hessian matrix, was employed \cite{hutchinson-method}. The Hutchinson method approximates the expected value of the quadratic form of the Hessian matrix and a Rademacher random vector—where each element takes the value of either $1$ or $-1$ with equal probability of $\frac{1}{2}$.

\begin{equation}
\begin{split}
\label{def:hessian_trace}
    \mathrm{tr}(H^{f}) = \mathrm{tr}(H^{f}I) = \mathrm{tr}(H^{f} \mathbb{E}[vv^{T}])\\=
    \mathbb{E}[\mathrm{tr}(H^{f} vv^{T})] = \mathbb{E}[v^{T}H^{f}v]
\end{split}
\end{equation}

The computation of spectral radius $A(H^f)$ was computed using the power iteration method. This computational approach ensures a balance between resource efficiency and computation accuracy, enabling the practical estimation of critical metrics within our experimental context.
