# Supplementary material for: Geometric Insights into Focal Loss: Reducing Curvature for Enhanced Model Calibration
Source: arXiv:2405.00442 source file (2024-05-01)
Supplement: Supplementary file 4 [file E_exp_results.tex]

% \clearpage
% \clearpage
\begin{figure}[t]
    \centering	
    \includegraphics[width=0.447\linewidth]{figs/fig4/Val/avg_val_acc-vs-avg_val_ece-20.pdf}\hspace{4mm}
    \includegraphics[width=0.447\linewidth]{figs/fig4/Test/avg_test_acc-vs-avg_test_ece-20.pdf}\\
    \includegraphics[width=0.447\linewidth]{figs/fig4/Val/avg_val_acc-vs-avg_val_ece-60.pdf}\hspace{4mm}
    \includegraphics[width=0.447\linewidth]{figs/fig4/Test/avg_test_acc-vs-avg_test_ece-60.pdf}\\
    \includegraphics[width=0.447\linewidth]{figs/fig4/Val/avg_val_acc-vs-avg_val_ece-100.pdf}\hspace{4mm}
    \includegraphics[width=0.447\linewidth]{figs/fig4/Test/avg_test_acc-vs-avg_test_ece-100.pdf}\\
    \includegraphics[width=0.447\linewidth]{figs/fig4/Val/avg_val_acc-vs-avg_val_ece-140.pdf}\hspace{4mm}
    \includegraphics[width=0.447\linewidth]{figs/fig4/Test/avg_test_acc-vs-avg_test_ece-140.pdf}\\
    \includegraphics[width=0.49\linewidth]{figs/fig4/Val/avg_val_acc-vs-avg_val_ece-180.pdf}
    \includegraphics[width=0.49\linewidth]{figs/fig4/Test/avg_test_acc-vs-avg_test_ece-180.pdf}
\caption{Comparative analysis of SAM and Focal Loss in CIFAR10 to CIFAR10.1 task. (left column) evaluating the IID validation data, the (right column) evaluating the OOD test data. 
Furthermore, the figure is divided into two tiers representing evaluations at the 20 epoch (top) and 180 epoch (bottom). The X-axis denotes ACC, while the Y-axis represents ECE. The color of each data point corresponds to SR(H) (= $A(H^f)$) value. Boundaries are color-coded to distinguish between the two methods, with Focal Loss delineated in orange and SAM in light blue.}
\label{fig:fig4}
\vspace{-3mm}
\end{figure}

\section{Omitted Results in Main Paper}
\label{appendix:E}
\subsection{Transition of Correlation between OOD ACC and ECE}

From \cref{fig:fig4}, we first note that the trends in both IID validation data and OOD test data are relatively consistent, although differences between Focal Loss and SAM become more apparent in the evaluation using OOD test data. Each data point in the figure indicates the performance achieved using different hyperparameters, $\rho$ for SAM, and $\gamma$ for Focal Loss.
Interestingly, the SR(H) (= $A(H^f)$) values that can be ultimately achieved do not drastically vary between the early and later stages of learning. However, we observe significant changes in ACC, with a trend of ECE deterioration over time.
When it comes to model selection, it seems that with Focal Loss, there is a trade-off between ACC and ECE improvement - one often comes at the expense of the other. In contrast, with SAM, improving ECE often leads to an enhancement in ACC, as we explained in the main paper (\cref{fig:fig1}).
Lastly, we note that while the smallest $A(H^f)$ is not always best for both ECE and ACC in both Focal Loss and SAM, it is clear that larger $A(H^f)$ values are undesirable in terms of ACC and ECE performance. This information presents valuable insight for further exploration of the optimal balance between these factors.

\begin{figure}[tb]
    \centering	
    \includegraphics[width=0.49\linewidth]{figs/fig5/test_tr_h-vs-avg_test_acc.pdf}
    \includegraphics[width=0.49\linewidth]{figs/fig5/test_tr_h-vs-avg_test_ece.pdf}

\caption{OOD Test Evaluation: Effects of batch size variations on the behavior of SAM in the CIFAR10.1 task. Each color represents an experiment with a different batch size. }
\label{fig:fig5}
\end{figure}

\begin{figure}[tb]
    \centering	
    \includegraphics[width=0.49\linewidth]{figs/fig6/train_tr_h-vs-avg_train_acc.pdf}
    \includegraphics[width=0.49\linewidth]{figs/fig6/train_tr_h-vs-avg_train_ece.pdf}

\caption{ID Train Evaluation: Effects of batch size variations on the behavior of SAM in the CIFAR10.1 task. Each color represents an experiment with a different batch size. }
\label{fig:fig6}
\end{figure}

\subsection{Ablation Study: Batch Size Comparison}

\Cref{fig:fig5} shows the figure shown as \cref{fig:fig3} on the main paper, evaluated in terms of $\mathrm{tr}(H^{f})$ instead of $A(H^f)$.
There is no significant difference between evaluation with $A(H^f)$ and with $\mathrm{tr}(H^{f})$, suggesting that the maximum eigenvalue is dominant.
Also, the smaller the $\mathrm{tr}(H^{f})$, the better the ACC and the higher the ECE tend to be.

\Cref{fig:fig6} shows the case of evaluation with training data. In this case, the trend is different from that of the case where OOD test data is used.
Specifically, when $\mathrm{tr}(H^{f})$ is sufficiently small or extremely large, high ACC is achieved, and low ECE is also achieved.
The BS=1 case tends to have a large $\mathrm{tr}(H^{f})$, but shows superior performance in terms of ID train ACC and ECE.
In contrast, the BS=Full case shows unfavorable performance in ACC and ECE.

\subsection{Additional Experiments: DomainBed Dataset}

\Cref{fig:fig7} shows the relationship between $\rho$, $A(H^f)$, and OOD test ACC in SAM for the DomainBed datasets (PACS \cite{li2017deeper}, VLCS \cite{fang2013unbiased}
, OffieHome \cite{venkateswara2017deep}, and DomainNet \cite{peng2019moment}
).
As with CIFAR10.1 and ImageNet-V2, $A(H^f)$ can be controlled by $\rho$, indicating that there is an appropriate $A(H^f)$ to achieve optimal OOD performance.

\begin{figure}[h]
    \centering	

    \includegraphics[width=0.49\linewidth]{figs/fig7/PACS-rho-vs-avg_test_eigen_h-5000.pdf}
    \includegraphics[width=0.49\linewidth]{figs/fig7/VLCS-rho-vs-avg_test_eigen_h-5000.pdf}
    \includegraphics[width=0.49\linewidth]{figs/fig7/OfficeHome-rho-vs-avg_test_eigen_h-5000.pdf}
    \includegraphics[width=0.49\linewidth]{figs/fig7/DomainNet-rho-vs-avg_test_eigen_h-5000.pdf}
\vspace{-3mm}
\caption{Impact of hyperparameters $\rho$ for SAM on the SR(H) in DomainBed dataset. Each data point represents an experiment with different $\rho$ values. As $\rho$ increases, SR(H) is generally reduced. However, while a larger $\gamma$ in Focal Loss results in a lower SR(H), it may lead to ACC deterioration if increased excessively. With SAM, an optimal $\rho$ is observed to yield the best ACC performance, as we already provide in the main paper (see \cref{fig:fig2}.)}
\label{fig:fig7}
\vspace{-5mm}
\end{figure}
